# Supplementary material for: READY or Not: Reliable Enterprise Agent Deployment
Source: arXiv:2609.02095 source file (2026-09-02)
Supplement: Supplementary file 1 [file appendix_a_contributor_form.tex]

\section{Contributor Submission Form}
\label{app:callform}

The contributor submission portal collects: (1) contributor expertise and years of experience, (2) industry, function, and professional role, (3) workflow name and business purpose, (4) frequency and typical human completion time, (5) decisions or downstream actions supported, (6) starting materials and systems, (7) tools normally used, (8) expected deliverable or final system state, (9) agent authority and prohibited actions, (10) policies and standards governing the task, (11) known ambiguities and escalation conditions, (12) common professional failure modes, (13) reference artifact or expert completion, (14) proposed evaluation criteria, (15) risk, reversibility, and potential impact, (16) data ownership and release permissions, and (17) public, private, or secure participation preference. No production data should be submitted without appropriate authorization, de-identification, and contractual controls.

The portal is implemented as a web form organized into seven sections: (A) contributor profile, (B) workflow overview, (C) inputs, tools, and deliverable, (D) agent authority and governance, (E) reference artifact and evaluation, (F) risk and data governance, and (G) participation role and attestation. Section~G additionally records the contributor's preferred participation role (domain adviser, task contributor, expert reviewer, enterprise design partner, or evaluation researcher) and requires an explicit data-policy attestation before submission.
