# Supplementary material for: READY or Not: Reliable Enterprise Agent Deployment
Source: arXiv:2609.02095 source file (2026-09-02)
Supplement: Supplementary file 2 [file appendix_b_roadmap.tex]

\section{Release Roadmap}
\label{app:roadmap}

The proposed release follows five phases. \emph{Phase 0 --- Freeze the construct:} deliver the multi-axis taxonomy, task schema, acceptance criteria, risk and authority model, contributor agreements, data policy, and deployment-profile specification; the public call should not launch before these are stable. \emph{Phase 1 --- Build the Tier-1 substrate:} contributor portal MVP, task registry, artifact sandbox, agent-run API, trace and artifact storage, and deterministic and rubric graders, seeded with existing finance, healthcare, and life-sciences workflows. \emph{Phase 2 --- Closed contributor pilot:} staff domain chairs, senior practitioners per vertical, evaluation engineers, data or security reviewers, and task editors; target 12--15 workflow families with 8--12 instances each ($\approx$120--180 validated instances), three repeated runs per configuration, and 6--8 baseline agents. \emph{Phase 3 --- Benchmark validation:} expert baseline completion, independent reference review, agent dry runs, evaluator calibration, false-positive and false-negative analysis, adversarial tests, a human-review-time study, and oversight-cost calculation. \emph{Phase 4 --- First release:} taxonomy and methodology paper, a $10$--$15\%$ public development set, a private evaluation pool, contributor and participant calls, an initial leaderboard, deployment profiles for baseline agents, and a task gallery with sanitized examples.
