# Supplementary material for: READY or Not: Reliable Enterprise Agent Deployment
Source: arXiv:2609.02095 source file (2026-09-02)
Supplement: Supplementary file 3 [file appendix_c_metrics.tex]

\section{Metric Families and Deployment Contract}
\label{app:metrics}

Enterprise's First Exam reports multiple metric families rather than a single score: \emph{outcome} (final-answer accuracy, task success, final-state and business-rule correctness, decision-artifact quality); \emph{grounding} (citation precision and recall, unsupported- and contradicted-claim rates, evidence sufficiency, source coverage); \emph{process} (tool-selection accuracy, retrieval quality, workflow-path correctness, unnecessary steps, error recovery, trace completeness); \emph{safety and compliance} (policy-violation, unauthorized-action, privacy-leakage, and jailbreak-success rates, escalation accuracy, approval-bypass rate); \emph{oversight cost} (human review time, correction rate and edit distance, escalation volume, approval burden, reviewer confidence, expected human cost per completed task, and oversight-cost reduction over model iterations); and \emph{operational} (latency, cost per task, tool-call efficiency, retry rate, failure recovery, robustness under changed state, and repeated-trial reliability). Aggregated per task and across tasks, these constitute the deployment contract summarized by the profile in \cref{lst:profile}: gate status, qualified tier, risk envelope, oversight policy, expected oversight cost, and an improvement path from failures to reduced review burden.
