# Supplementary material for: READY or Not: Reliable Enterprise Agent Deployment
Source: arXiv:2609.02095 source file (2026-09-02)
Supplement: Supplementary file 4 [file appendix_d_example_tasks.tex]

\section{Example Enterprise's First Exam Tasks}
\label{app:tasks}

\paragraph{Tier 1 --- Due-diligence agent.} Given a virtual data room (financial statements, customer contracts, board materials, sales-pipeline exports, management presentations), the agent produces a diligence memo identifying revenue-concentration risk: retrieve evidence across documents and spreadsheets, identify top customers and revenue contribution, compare management claims against source data, detect missing or inconsistent information, produce a cited memo, and escalate unresolved contradictions. Evaluation covers factual accuracy, source grounding, completeness, contradiction handling, abstention quality, and decision relevance.

\paragraph{Tier 1 --- Patient-safety event review agent.} Reviewing adverse-event reports, clinical notes, product-complaint records, and prior safety signals, the agent determines whether an event should be escalated for human safety review (the running example of \cref{lst:taskrecord}): retrieve case evidence, summarize the event timeline, identify missing information, compare against reporting criteria, surface uncertainty, and recommend escalation when warranted. Evaluation covers evidence coverage, medical and regulatory grounding, missing-information detection, escalation correctness, and hallucination avoidance.

\paragraph{Tier 2 --- Procure-to-pay reconciliation agent.} Given a vendor statement, the agent reconciles it against ERP invoice and payment records; on a likely overpayment or credit it creates a case, attaches evidence, drafts a vendor communication, and routes for approval, while avoiding unauthorized financial actions. Evaluation covers extraction accuracy, reconciliation correctness, final system state, write-action safety, auditability, and human-review quality.

\paragraph{Tier 2 --- IT service-management agent.} Given an internal support ticket about an access issue, the agent inspects the user's role, relevant permissions, and standard operating procedure, updates the ticket, and triggers the correct access workflow, avoiding unauthorized provisioning and routing high-risk requests for approval. Evaluation covers policy compliance, permission handling, correct workflow state, escalation correctness, and idempotency.

\paragraph{Tier 3 --- Customer-service refund agent.} A customer requests a refund; the agent must understand the issue, retrieve order information, apply refund policy, ask for missing information, resist out-of-policy exceptions, and either process the refund or escalate. Evaluation covers task success, policy compliance, conversation quality, tool-use correctness, safety, and user experience.

\paragraph{Tier 3 --- Telecom technical-support agent.} In a dual-control setting, the agent checks account and service state while the user performs device troubleshooting; it must diagnose through conversation, guide the user, interpret user-reported observations, use tools to inspect service state, avoid unsafe account changes, and escalate when unresolved. Evaluation covers dual-control coordination, conversation robustness, instruction clarity, policy compliance, and repeated-trial reliability.
